# Supplementary material for: Optimum-statistical Collaboration Towards General and Efficient Black-box Optimization
Source: arXiv:2106.09215 source file (2023-05-31)
Supplement: Supplementary file 1 [file appendixE.tex]

% \section{Discussions on the Parameter-Agnosticity}
% \label{app: VPCT}


% \input{Sections/01.01.Table}

% In this subsection, we discuss the $\mathtt{VPCT}$ algorithm, which is the parameter-agnostic version of $\mathtt{VHCT}$. We first present the algorithm as in Algorithm \ref{alg: VPCT}. Note that it utilizes the $\OurAlg$ (Algorithm \ref{alg: VHCT}) proposed in Section \ref{sec: algo_theo} and the $\mathtt{POO}$ algorithm \citep{Grill2015Blackbox}.


% \begin{remark}\textbf{(Parameter-agnostic $\mathtt{VHCT}$)}. Note that any base algorithm with a desirable cumulative regret upper bound under the local smoothness assumption can be used as a subroutine for the meta algorithm \texttt{POO} \citep{shang2019general}. Therefore, \texttt{POO}($\OurAlg$), which we refer to as \texttt{VPCT}, is guaranteed to have a variance-dependent simple regret bound of size $\mathcal{O} (V_{\max}^{{1}/({d+2})}  (\log^2 n/n)^{1/(d+2)} )$. Compared with the simple regret bound of $\OurAlg$ with known smoothness parameters, the bound of \texttt{VPCT} is only worse by a logarithmic factor $(\log n)^{1/(d+2)}$. However, \texttt{VPCT} is parameter-agnostic since the meta-algorithm \texttt{POO} can tune the smoothness parameters automatically. We provide the corresponding algorithm and its theoretical analysis in Appendix \ref{app: VPCT}.
% \end{remark}





% \begin{algorithm}[ht]
%   \caption{ $\mathtt{VPCT}$: Variance-adaptive Parallel High Confidence Tree}
%   \label{alg: VPCT}
% \begin{algorithmic}[1]
%   \STATE \textbf{Input:} $\rho_{\max }, \nu_{\max}$
%   \STATE \textbf{Initialization:} $D_{\max } \leftarrow \ln K / \ln \left(1 / \rho_{\max }\right)$, $n \leftarrow 0$, $N \leftarrow 1, \mathcal{S} \leftarrow\left\{\left(\nu_{\max }, \rho_{\max }\right)\right\}$
%   \WHILE{\textit{budget still available }}
%   \WHILE{$N \leq \frac{1}{2} D_{\max} \log(n/\log n)$}
%   \FOR{ $i \leftarrow 1, \ldots, N$}
%   \STATE $ s \leftarrow (\nu_{\max}, \rho_{\max}^{(2N/(2i+1)})$
%   \STATE Initialize $\mathtt{VHCT}$ with parameters $s$
%   \STATE Obtain $n/N$ rewards $r_{s,1}, r_{s,2}, \ldots, r_{s,n/N}$
%   \STATE Compute the average reward $\hat{\mu}[s] = \frac{N}{n} \sum_{i=1}^{n/N} r_{s,i}$
%   \ENDFOR
%   \STATE $n\leftarrow 2n, N \leftarrow 2N$
%   \ENDWHILE
%   \STATE Perform each initialized $\mathtt{VHCT}(s)$ once and update the average $\hat{\mu}[s]$
%   \STATE $n \leftarrow n+N$
%   \ENDWHILE
%   \STATE $s^* \leftarrow \text{argmax}_{s\in \mathcal{S}}\hat{\mu}[s]$
%   \RETURN
% \end{algorithmic}
% \end{algorithm}

% Now we provide the simple regret bound of $\mathtt{VPCT}$ in Theorem \ref{Thm: VPCT_regret_bound}.
% \begin{theorem}
% \label{Thm: VPCT_regret_bound}
% Assume that the objective function $f$ satisfies condition (\ref{eq:local_smoothness}). The simple regret of Algorithm \ref{alg: VPCT} is upper bounded by
% \begin{equation}
% \nonumber
%   \mathbb{E}[S^{\mathtt{VHCT}}_n] = \mathcal{O} \left(V_{\max}^{\frac{1}{d+2}}  (\log^2 n /n)^{1/(d+2)} \right)
% \end{equation}
% \end{theorem}


% The above single regret bound also depends on the maximum variance in history, which is desirable since it would be small when the variance is small. Therefore, we conclude our analysis with the claim that both $\mathtt{VHCT}$ and $\mathtt{VPCT}$ can converge faster than the non-adaptive algorithms. 


% \subsection{Discussions}
% \textbf{Comparison with $\mathtt{HOO}$ and $\mathtt{HCT}$}. Although all three algorithms rely on the concept of \textit{upper-confidence bounds} (UCBs) for collaborative optimism, we are the first work that clearly explains the interaction between the resolution descriptor and the uncertainty quantifier, and how the statistical optimum end-goal is achieved. Our choice of the uncertainty quantifier $\mathtt{SE}_{h,i}(t)$ is the first one to utilize the variance information when measuring the statistical error and thus our algorithm converges faster when the noise is small. $\mathtt{HOO}$ and $\mathtt{HCT}$ do not adapt to different noises because their strategies of the collaboration between $\mathtt{OE}$ and $\mathtt{SE}$ are defined in advance. For example, the algorithm of $\mathtt{HCT}$ also uses a threshold for tree expansion when $\mathtt{OE} \approx \mathtt{SE}$ , but they define $\tau_h(t) ={\mathcal{O}}((\rho^{h}\nu)^{-2}b^2 \log (t))$ for all the nodes on level $h$, which is fixed when the parameters are fixed. In other words, the number of pulls needed to expand a node $\mathcal{P}_{h,i}$ at time $t$ is always the same regardless of the noise complexity. Our unique choice of the uncertainty quantifier determines that our $\tau_{h,i}(t)$s are node-specific and they are able to adapt to different noises. Although the cumulative regret bounds of these algorithms are all of order $\mathcal{O}(n^{(d+1)/(d+2)}\log n^{1/(d+2)})$, our regret bound depends on the maximum variance in the optimization process, and thus we expect $\OurAlg$ to be faster than $\mathtt{HOO}$ and $\mathtt{HCT}$ when the noise is small or moderate.

% \textbf{Comparison with $\mathtt{StroquOOL}$}.
% Both $\OurAlg$ and $\mathtt{StroquOOL}$ can adapt to different levels of noises, and interestingly we have found that their dependence on the maximum variance is the same, i.e., the regret bounds of these two algorithms both scale with $V_{\max}^{1/(d+2)}$. However, $\mathtt{StroquOOL}$ is not an anytime algorithm because it needs to know the budget $n$ in advance as an input parameter. Also, \citet{bartlett2019simple} require the budget $n$ to be larger than a threshold in the high-noise regime (Corollary 9 in the $\mathtt{StroquOOL}$ paper), which is an extra condition that we don't need. Moreover, only simple regret bound is provided in the paper of $\mathtt{StroquOOL}$ while we provide both simple and cumulative regret bounds. The advantage of $\mathtt{StroquOOL}$ in the stochastic setting is that it does not need the smoothness parameters $(\rho, \nu)$, but we can simply run the agnostic version $\mathtt{VPCT}$ when parameter tuning is not preferred. The simple regret bound of $\mathtt{VPCT}$ is  logarithmically better than the bound of  $\mathtt{StroquOOL}$ since $ \mathbb{E}(S_n^{\mathtt{VPCT}}) = \mathcal{O}( \log(n)^2/n)^{1/(d+2)}) \leq \mathcal{O}( \log(n)^3/n)^{1/(d+2)}) =  \mathbb{E}(S_n^{\mathtt{StroquOOL}})$ and it is still an anytime algorithm (Table \ref{tab: summary}).


% \subsection{Proof of Theorem \ref{Thm: VPCT_regret_bound}}
% \textbf{Proof}. The proof follows the original proof of $\mathtt{POO}$, but taking advantage of the cumulative regret bound we have proved in Theorem \ref{Thm: regret_bound}. Note that by the grid search strategy of $\mathtt{POO}$, Lemma \ref{lem: distance_between_dimension} ensures that for $\rho_i$ in the grid, the following quantity
% \begin{equation}
%     \nonumber
%     \bar{\rho} := \underset{\rho_{i} \geq \rho^{\star}}{\arg \min }\left[d\left(\nu_{\max }, C_{i}, \rho_{i}\right)-d\left(\nu^{\star}, C^{\star}, \rho^{\star}\right)\right]
% \end{equation}
% satisfies $d\left(\nu_{\max }, \bar{C}, \bar{\rho}\right)-d\left(\nu^{\star}, C^{\star}, \rho^{\star}\right) \leq D_{\max } / N$, where $\bar{C}$ is the constant associated to $\bar{\rho}$. Therefore note that we have cumulative regret upper bound in Theorem \ref{Thm: regret_bound}, we have the following simple regret bound by following the Appendix B.2 and B.3 of \citet{Grill2015Blackbox}.

% \begin{equation}
%     \nonumber
% \log \mathbb{E}\left[ S_n^{\mathtt{VPCT}}\right] \leq \log C_1 V_{\max}^{\frac{1}{d+2}}   +\frac{\log \bar{C}}{d\left(\bar{\rho}\right)+2} + \log \left(\frac{\log \lfloor n/N \rfloor}{\lfloor n/N \rfloor} \right) \left(\frac{1}{2 + d(\rho^*)}- \frac{D_{\max} /N}{(2+d(\rho^*))^2}\right)
% \end{equation}

% Now since $N \leq D_{\max} \log (n/\log n)$, we have 

% \begin{equation}
%     \nonumber
%     \log \left(\frac{\log \lfloor n/N \rfloor}{\lfloor n/N \rfloor} \right) \leq \log (D_{\max} \log n \log (n/\log n)/n) \leq \log (D_{\max} \log^2 n/n)
% \end{equation}

% Also the second term can be bounded by $\gamma + \frac{D_{\max}}{2+d(\rho^*)} \log (\nu_{\max}/\nu^*)$ for some constant $\gamma$. The last term can also be bounded by 

% \begin{equation}
%     \nonumber
% -\log \left(\frac{\log \lfloor n/N \rfloor}{\lfloor n/N \rfloor} \right)  \frac{D_{\max} /N}{(2+d(\rho^*))^2}\leq \log \left ( \frac{n}{D_{\max}\log n \log(n/\log n)} \right) \frac{1}{ 2\log(n/\log n)}  \leq 2
% \end{equation}


% Therefore we can finally bound the simple regret of $\mathtt{VPCT}$ by 


% \begin{equation}
% \nonumber
%   \begin{aligned}
% \mathbb{E}\left[S_{n}^{\mathtt{VPCT}}\right]
% &\leq C_1 V_{\max}^{\frac{1}{d+2}}  \exp(\gamma+2) D_{\max } \left(\nu_{\max } / \nu^{\star}\right)^{D_{\max }} (\log ^{2} n / n)^{1 /(d(\rho^{\star})+2} \\
% & = \mathcal{O}\left( V_{\max}^{\frac{1}{d+2}}   (\log^{2} n / n )^{d+2} \right)
% \end{aligned}
% \end{equation}

% Now since the empirical best instance we choose at the final step is not far from $\bar{\rho}$, i.e., the additional regret at the final step is a constant \citep{Grill2015Blackbox}. We conclude that the regret bound of $\mathtt{VPCT}$ is $\mathcal{O}\left( V_{\max}^{\frac{1}{d+2}}  (\log^{2} n / n )^{d+2} \right)$ \hfill $\square$


% \begin{lemma}
% \label{lem: distance_between_dimension}
% \textbf{\upshape (Appendix B.1 of \citet{Grill2015Blackbox})} Under Equation \ref{eq:local_smoothness}, for any choice of $\rho^{\star}$ and $\rho$ s.t. $0<\rho^{\star}<\rho<1$, we have
% $$
% d\left(\nu_{\max }, C, \rho\right)-d\left(\nu^{\star}, C^{\star}, \rho^{\star}\right) \leq \log K\left(\frac{1}{\log (1 / \rho)}-\frac{1}{\log \left(1 / \rho^{\star}\right)}\right)
% $$
% \end{lemma}
